# Supplementary material for: Influence of Tissue Geometry on Transversal Relaxation
Source: arXiv:1305.6258 source file (2013-05-27)
Supplement: Supplementary file 1 [file Appendix_ICD.tex]

\chapter{Tabellarische Auflistung für verschiedene Modelle}\label{appendix:icd}
Noch auszufüllen...\newline
	\begin{table}[H]
		
		\begin{center}
		\begin{tabular}[ht]{l|c|c|ccc|ccc} 		

		$\dom_0$ & $\eta$ 			& $\ICD [\mum]$		&	$R_{2,min}^*$ & $R_{2,avg}^*$ &	$R_{2,max}^*$ & $T_{2,min}^*$ & $T_{2,avg}^*$ &	$T_{2,max}^*$ \\
		\hline
		\hline
		\multirow{3}{1cm}{\begin{sideways}\parbox{2.5cm}{$\displaystyle(150\pm50)\radps$}\end{sideways}}
						& $ (7\pm1)\%$	&	 18.4						&		17.3			& 20.7				& 26.9				&	37.1 				& 48.3 				& 57.8 			\\[1.5ex]
						& $(12\pm1)\%$	&	 13.9						&		17.7			&	21.8				& 29.1				& 34.4				&	45.9				& 56.5 			\\[1.5ex]
						& $(17\pm1)\%$	&	 11.6						&		18.1			& 22.7				& 31.1				& 32.1				&	44.1				& 55.4			\\[1.5ex]
		\hline
		\multirow{3}{1cm}{\begin{sideways}\parbox{2.8cm}{$\displaystyle(750\pm250)\radps$}\end{sideways}}
						& $ (7\pm1)\%$	&	 18.4						&		29.9			& 56.4				& 94.4				&	10.6				& 17.7				& 33.4			\\[1.5ex]
						& $(12\pm1)\%$	&	 13.9						&		37.7			&	73.9				& 127.7				&	7.8					&	13.5				& 26.5			\\[1.5ex]
						& $(17\pm1)\%$	&	 11.6						&		44.2			&	87.3				& 152.6				&	6.6					&	11.5				& 22.6			\\[1.5ex]
		\end{tabular}
		\end{center}
		\caption{Aus Simulationen bestimmte Relaxationszeiten für das hex. Gitter($\Gamma=\infty$).\newline
		Relaxationsraten sind in $s^{-1}$, Relaxationszeiten in $\ms$ gegeben.}
		\label{tab:hex-Relaxations-icd}
	\end{table}
	
	\begin{table}
		
		\begin{center}
		\begin{tabular}[ht]{l|c|c|ccc|ccc} 		

		$\dom_0$ & $\eta$ 			& $\ICD [\mum]$		&	$R_{2,min}^*$ & $R_{2,avg}^*$ &	$R_{2,max}^*$ & $T_{2,min}^*$ & $T_{2,avg}^*$ &	$T_{2,max}^*$ \\
		\hline
		\hline
		\multirow{3}{1cm}{\begin{sideways}\parbox{2.5cm}{$\displaystyle(150\pm50)\radps$}\end{sideways}}
						& $ (7\pm1)\%$	&	 18.4						&		17.3			& 20.7				& 26.9				&	37.1 				& 48.3 				& 57.8 			\\[1.5ex]
						& $(12\pm1)\%$	&	 13.9						&		17.7			&	21.8				& 29.1				& 34.4				&	45.9				& 56.5 			\\[1.5ex]
						& $(17\pm1)\%$	&	 11.6						&		18.1			& 22.7				& 31.1				& 32.1				&	44.1				& 55.4			\\[1.5ex]
		\hline
		\multirow{3}{1cm}{\begin{sideways}\parbox{2.8cm}{$\displaystyle(750\pm250)\radps$}\end{sideways}}
						& $ (7\pm1)\%$	&	 18.4						&		29.9			& 56.4				& 94.4				&	10.6				& 17.7				& 33.4			\\[1.5ex]
						& $(12\pm1)\%$	&	 13.9						&		37.7			&	73.9				& 127.7				&	7.8					&	13.5				& 26.5			\\[1.5ex]
						& $(17\pm1)\%$	&	 11.6						&		44.2			&	87.3				& 152.6				&	6.6					&	11.5				& 22.6			\\[1.5ex]
		\end{tabular}
		\end{center}
		\caption{Aus Simulationen bestimmte Relaxationszeiten für das Krogh-Modell.\newline
		Relaxationsraten sind in $s^{-1}$, Relaxationszeiten in $\ms$ gegeben.}
		\label{tab:krogh-Relaxations-icd}
	\end{table}
	
	\begin{table}
		
		\begin{center}
		\begin{tabular}[ht]{l|c|c|ccc|ccc} 		

		$\dom_0$ & $\eta$ 			& $\ICD [\mum]$		&	$R_{2,min}^*$ & $R_{2,avg}^*$ &	$R_{2,max}^*$ & $T_{2,min}^*$ & $T_{2,avg}^*$ &	$T_{2,max}^*$ \\
		\hline
		\hline
		\multirow{3}{1cm}{\begin{sideways}\parbox{2.5cm}{$\displaystyle(150\pm50)\radps$}\end{sideways}}
						& $ (7\pm1)\%$	&	 18.4						&		17.3			& 20.7				& 26.9				&	37.1 				& 48.3 				& 57.8 			\\[1.5ex]
						& $(12\pm1)\%$	&	 13.9						&		17.7			&	21.8				& 29.1				& 34.4				&	45.9				& 56.5 			\\[1.5ex]
						& $(17\pm1)\%$	&	 11.6						&		18.1			& 22.7				& 31.1				& 32.1				&	44.1				& 55.4			\\[1.5ex]
		\hline
		\multirow{3}{1cm}{\begin{sideways}\parbox{2.8cm}{$\displaystyle(750\pm250)\radps$}\end{sideways}}
						& $ (7\pm1)\%$	&	 18.4						&		29.9			& 56.4				& 94.4				&	10.6				& 17.7				& 33.4			\\[1.5ex]
						& $(12\pm1)\%$	&	 13.9						&		37.7			&	73.9				& 127.7				&	7.8					&	13.5				& 26.5			\\[1.5ex]
						& $(17\pm1)\%$	&	 11.6						&		44.2			&	87.3				& 152.6				&	6.6					&	11.5				& 22.6			\\[1.5ex]
		\end{tabular}
		\end{center}
		\caption{Aus Simulationen bestimmte Relaxationszeiten nach Strong-Kollision-Approximation.\newline
		Relaxationsraten sind in $s^{-1}$, Relaxationszeiten in $\ms$ gegeben.}
		\label{tab:sc-Relaxations-icd}
	\end{table}
